# Supplementary material for: ORB5: a global electromagnetic gyrokinetic code using the PIC approach in toroidal geometry
Source: arXiv:1905.01906 source file (2019-05-06)
Supplement: Supplementary file 1 [file appendix.tex]

%%% Local Variables:
%%% mode: latex
%%% TeX-master: "../ORB5Review"
%%% End:
